# Supplementary material for: Motion-Based Generator Model: Unsupervised Disentanglement of Appearance, Trackable and Intrackable Motions in Dynamic Patterns
Source: arXiv:1911.11294 source file (2019-11-26)
Supplement: Supplementary file 1 [file supplementary.tex]

\section{More results}

\subsection{More results on generating image from architectural labels for Section 4.2.1}
Figure \ref{fig:supp_building1}, \ref{fig:supp_building2}, \ref{fig:supp_building3}, and \ref{fig:supp_building4} show more results of generating images conditioned on architectural labels with higher resolution. The first column displays semantic label images that are unseen in the training data as conditions. The second column shows the ground truth images corresponding to the condition images. The third columns show the resluts generated by the baseline method pixel2pixel \cite{isola2017image}. The fourth and fifth columns are the results generated by the policy-like model and the planner-like model respectively. The input and the output images are of the size $256 \times 256$ pixels.  

\subsection{More results on generating face images from sketch images for Section 4.2.2}

Figure \ref{fig:supp_face} shows more results of condition interpolation for the experiment in Section 4.2.2. For each row, the color face images are generated by interpolating between the embedding of the sketch images shown at two ends. Even though we don't observe the sketch images that corresponds to the generated images at the intervening points, the learned encoder $\Phi(C)$ for condition embedding has captured a smooth manifold for the sketch images, such that we can generate realistic face images conditioned on a series of linearly interpolated sketch images embedding. For each row, you see one face shown at the left end slowly being transformed into the other face shown at the right end.

\subsection{More results on shoe generation from edge image for Section 4.2.2}
Figure \ref{fig:supp_boot} shows more results of generating shoe images from the corresponding edge images extracted by HED edge detector \cite{xie2015holistically} with post processing for the experiment discussed in Section 4.2.2. The top panel displays the edge images, while the bottom panel displays the generated shoe images by the planner-like model. 

\subsection{More results on image inpainting for Section 4.2.3}

Figure \ref{fig:supp_recovery} shows more results on the experiment of image inpainting in Section 4.2.3. The first column displays the testing images ($256 \times 256$ pixels) with a hole of $128 \times 128$ that need to be inpainted. The second column shows the ground truth as reference. The rest three columns respectively display the inpainted results by the pixel2pixel method \cite{isola2017image}, the policy-like model, and the planner-like model. The method proposed in this paper, which is a framework with the cooperatively trained policy-like model and planner-like model, can obtain more reasonably realistic inpainting results (shown at the last column) than those by the baseline method.

\begin{figure*}[h]
\centering
\hspace{2mm} Condition \hspace{24mm} GT \hspace{20mm} pixel2pixel \hspace{20mm} policy-like \hspace{14mm} planner-like \\
\includegraphics[width=.19\linewidth]{./results/CMP_new/synthesis_test/test_004_src.png}
\includegraphics[width=.19\linewidth]{./results/CMP_new/CMP_test/test/test_004_tgt.png}
\includegraphics[width=.19\linewidth]{./results/CMP_new/facades_pix2pix/images/5_fake_B.png}
\includegraphics[width=.19\linewidth]{./results/CMP_new/CMP_test/test/test_004_gen.png} \includegraphics[width=.19\linewidth]{./results/CMP_new/synthesis_test/test_004_des.png}\\ \vspace{1mm}
\includegraphics[width=.19\linewidth]{./results/CMP_new/synthesis_test/test_005_src.png}
\includegraphics[width=.19\linewidth]{./results/CMP_new/CMP_test/test/test_005_tgt.png}
\includegraphics[width=.19\linewidth]{./results/CMP_new/facades_pix2pix/images/6_fake_B.png}
\includegraphics[width=.19\linewidth]{./results/CMP_new/CMP_test/test/test_005_gen.png} \includegraphics[width=.19\linewidth]{./results/CMP_new/synthesis_test/test_005_des.png}\\ \vspace{1mm}
\includegraphics[width=.19\linewidth]{./results/CMP_new/synthesis_test/test_007_src.png}
\includegraphics[width=.19\linewidth]{./results/CMP_new/CMP_test/test/test_007_tgt.png}
\includegraphics[width=.19\linewidth]{./results/CMP_new/facades_pix2pix/images/8_fake_B.png}
\includegraphics[width=.19\linewidth]{./results/CMP_new/CMP_test/test/test_007_gen.png} \includegraphics[width=.19\linewidth]{./results/CMP_new/synthesis_test/test_007_des.png}\\ \vspace{1mm}
\includegraphics[width=.19\linewidth]{./results/CMP_new/synthesis_test/test_037_src.png}
\includegraphics[width=.19\linewidth]{./results/CMP_new/CMP_test/test/test_037_tgt.png}
\includegraphics[width=.19\linewidth]{./results/CMP_new/facades_pix2pix/images/38_fake_B.png}
\includegraphics[width=.19\linewidth]{./results/CMP_new/CMP_test/test/test_037_gen.png} \includegraphics[width=.19\linewidth]{./results/CMP_new/synthesis_test/test_037_des.png}\\ \vspace{1mm}
\includegraphics[width=.19\linewidth]{./results/CMP_new/synthesis_test/test_223_src.png}
\includegraphics[width=.19\linewidth]{./results/CMP_new/CMP_test/test/test_223_tgt.png}
\includegraphics[width=.19\linewidth]{./results/CMP_new/facades_pix2pix/images/224_fake_B.png}
\includegraphics[width=.19\linewidth]{./results/CMP_new/CMP_test/test/test_223_gen.png}
\includegraphics[width=.19\linewidth]{./results/CMP_new/synthesis_test/test_223_des.png} \\ \vspace{1mm}
\includegraphics[width=.19\linewidth]{./results/CMP_new/synthesis_test/test_011_src.png}
\includegraphics[width=.19\linewidth]{./results/CMP_new/CMP_test/test/test_011_tgt.png}
\includegraphics[width=.19\linewidth]{./results/CMP_new/facades_pix2pix/images/12_fake_B.png}
\includegraphics[width=.19\linewidth]{./results/CMP_new/CMP_test/test/test_011_gen.png}
\includegraphics[width=.19\linewidth]{./results/CMP_new/synthesis_test/test_011_des.png} \\ \vspace{1mm}
\caption{Generating images conditioned on architectural labels}	
\label{fig:supp_building1}
\end{figure*}

\begin{figure*}[h]
\centering
\hspace{2mm} Condition \hspace{24mm} GT \hspace{20mm} pixel2pixel \hspace{20mm} policy-like \hspace{14mm} planner-like \\
\includegraphics[width=.19\linewidth]{./results/CMP_new/synthesis_test/test_012_src.png}
\includegraphics[width=.19\linewidth]{./results/CMP_new/CMP_test/test/test_012_tgt.png}
\includegraphics[width=.19\linewidth]{./results/CMP_new/facades_pix2pix/images/13_fake_B.png}
\includegraphics[width=.19\linewidth]{./results/CMP_new/CMP_test/test/test_012_gen.png} \includegraphics[width=.19\linewidth]{./results/CMP_new/synthesis_test/test_012_des.png}\\ \vspace{1mm}
\includegraphics[width=.19\linewidth]{./results/CMP_new/synthesis_test/test_013_src.png}
\includegraphics[width=.19\linewidth]{./results/CMP_new/CMP_test/test/test_013_tgt.png}
\includegraphics[width=.19\linewidth]{./results/CMP_new/facades_pix2pix/images/14_fake_B.png}
\includegraphics[width=.19\linewidth]{./results/CMP_new/CMP_test/test/test_013_gen.png} \includegraphics[width=.19\linewidth]{./results/CMP_new/synthesis_test/test_013_des.png}\\ \vspace{1mm}
\includegraphics[width=.19\linewidth]{./results/CMP_new/synthesis_test/test_016_src.png}
\includegraphics[width=.19\linewidth]{./results/CMP_new/CMP_test/test/test_016_tgt.png}
\includegraphics[width=.19\linewidth]{./results/CMP_new/facades_pix2pix/images/17_fake_B.png}
\includegraphics[width=.19\linewidth]{./results/CMP_new/CMP_test/test/test_016_gen.png} \includegraphics[width=.19\linewidth]{./results/CMP_new/synthesis_test/test_016_des.png}\\ \vspace{1mm}
\includegraphics[width=.19\linewidth]{./results/CMP_new/synthesis_test/test_026_src.png}
\includegraphics[width=.19\linewidth]{./results/CMP_new/CMP_test/test/test_026_tgt.png}
\includegraphics[width=.19\linewidth]{./results/CMP_new/facades_pix2pix/images/27_fake_B.png}
\includegraphics[width=.19\linewidth]{./results/CMP_new/CMP_test/test/test_026_gen.png} \includegraphics[width=.19\linewidth]{./results/CMP_new/synthesis_test/test_026_des.png}\\ \vspace{1mm}
\includegraphics[width=.19\linewidth]{./results/CMP_new/synthesis_test/test_029_src.png}
\includegraphics[width=.19\linewidth]{./results/CMP_new/CMP_test/test/test_029_tgt.png}
\includegraphics[width=.19\linewidth]{./results/CMP_new/facades_pix2pix/images/30_fake_B.png}
\includegraphics[width=.19\linewidth]{./results/CMP_new/CMP_test/test/test_029_gen.png}
\includegraphics[width=.19\linewidth]{./results/CMP_new/synthesis_test/test_029_des.png} \\ \vspace{1mm}
\includegraphics[width=.19\linewidth]{./results/CMP_new/synthesis_test/test_036_src.png}
\includegraphics[width=.19\linewidth]{./results/CMP_new/CMP_test/test/test_036_tgt.png}
\includegraphics[width=.19\linewidth]{./results/CMP_new/facades_pix2pix/images/37_fake_B.png}
\includegraphics[width=.19\linewidth]{./results/CMP_new/CMP_test/test/test_036_gen.png}
\includegraphics[width=.19\linewidth]{./results/CMP_new/synthesis_test/test_036_des.png} \\ \vspace{1mm}
\caption{Generating images conditioned on architectural labels}	
\label{fig:supp_building2}
\end{figure*}

\begin{figure*}[h]
\centering
\hspace{2mm} Condition \hspace{24mm} GT \hspace{20mm} pixel2pixel \hspace{20mm} policy-like \hspace{14mm} planner-like \\
\includegraphics[width=.19\linewidth]{./results/CMP_new/synthesis_test/test_040_src.png}
\includegraphics[width=.19\linewidth]{./results/CMP_new/CMP_test/test/test_040_tgt.png}
\includegraphics[width=.19\linewidth]{./results/CMP_new/facades_pix2pix/images/41_fake_B.png}
\includegraphics[width=.19\linewidth]{./results/CMP_new/CMP_test/test/test_040_gen.png} \includegraphics[width=.19\linewidth]{./results/CMP_new/synthesis_test/test_040_des.png}\\ \vspace{1mm}
\includegraphics[width=.19\linewidth]{./results/CMP_new/synthesis_test/test_049_src.png}
\includegraphics[width=.19\linewidth]{./results/CMP_new/CMP_test/test/test_049_tgt.png}
\includegraphics[width=.19\linewidth]{./results/CMP_new/facades_pix2pix/images/50_fake_B.png}
\includegraphics[width=.19\linewidth]{./results/CMP_new/CMP_test/test/test_049_gen.png} \includegraphics[width=.19\linewidth]{./results/CMP_new/synthesis_test/test_049_des.png}\\ \vspace{1mm}

\includegraphics[width=.19\linewidth]{./results/CMP_new/synthesis_test/test_062_src.png}
\includegraphics[width=.19\linewidth]{./results/CMP_new/CMP_test/test/test_062_tgt.png}
\includegraphics[width=.19\linewidth]{./results/CMP_new/facades_pix2pix/images/63_fake_B.png}
\includegraphics[width=.19\linewidth]{./results/CMP_new/CMP_test/test/test_062_gen.png} \includegraphics[width=.19\linewidth]{./results/CMP_new/synthesis_test/test_062_des.png}\\ \vspace{1mm}
\includegraphics[width=.19\linewidth]{./results/CMP_new/synthesis_test/test_099_src.png}
\includegraphics[width=.19\linewidth]{./results/CMP_new/CMP_test/test/test_099_tgt.png}
\includegraphics[width=.19\linewidth]{./results/CMP_new/facades_pix2pix/images/100_fake_B.png}
\includegraphics[width=.19\linewidth]{./results/CMP_new/CMP_test/test/test_099_gen.png} \includegraphics[width=.19\linewidth]{./results/CMP_new/synthesis_test/test_099_des.png}\\ \vspace{1mm}

\includegraphics[width=.19\linewidth]{./results/CMP_new/synthesis_test/test_145_src.png}
\includegraphics[width=.19\linewidth]{./results/CMP_new/CMP_test/test/test_145_tgt.png}
\includegraphics[width=.19\linewidth]{./results/CMP_new/facades_pix2pix/images/146_fake_B.png}
\includegraphics[width=.19\linewidth]{./results/CMP_new/CMP_test/test/test_145_gen.png}
\includegraphics[width=.19\linewidth]{./results/CMP_new/synthesis_test/test_145_des.png} \\ \vspace{1mm}
\includegraphics[width=.19\linewidth]{./results/CMP_new/synthesis_test/test_146_src.png}
\includegraphics[width=.19\linewidth]{./results/CMP_new/CMP_test/test/test_146_tgt.png}
\includegraphics[width=.19\linewidth]{./results/CMP_new/facades_pix2pix/images/147_fake_B.png}
\includegraphics[width=.19\linewidth]{./results/CMP_new/CMP_test/test/test_146_gen.png}
\includegraphics[width=.19\linewidth]{./results/CMP_new/synthesis_test/test_146_des.png} \\ \vspace{1mm}
\caption{Generating images conditioned on architectural labels}	
\label{fig:supp_building3}
\end{figure*}

\begin{figure*}[h]
\centering
\hspace{2mm} Condition \hspace{24mm} GT \hspace{20mm} pixel2pixel \hspace{20mm} policy-like \hspace{14mm} planner-like \\
\includegraphics[width=.19\linewidth]{./results/CMP_new/synthesis_test/test_218_src.png}
\includegraphics[width=.19\linewidth]{./results/CMP_new/CMP_test/test/test_218_tgt.png}
\includegraphics[width=.19\linewidth]{./results/CMP_new/facades_pix2pix/images/219_fake_B.png}
\includegraphics[width=.19\linewidth]{./results/CMP_new/CMP_test/test/test_218_gen.png} \includegraphics[width=.19\linewidth]{./results/CMP_new/synthesis_test/test_218_des.png}\\ \vspace{1mm}
\includegraphics[width=.19\linewidth]{./results/CMP_new/synthesis_test/test_224_src.png}
\includegraphics[width=.19\linewidth]{./results/CMP_new/CMP_test/test/test_224_tgt.png}
\includegraphics[width=.19\linewidth]{./results/CMP_new/facades_pix2pix/images/225_fake_B.png}
\includegraphics[width=.19\linewidth]{./results/CMP_new/CMP_test/test/test_224_gen.png} \includegraphics[width=.19\linewidth]{./results/CMP_new/synthesis_test/test_224_des.png}\\ \vspace{1mm}

\includegraphics[width=.19\linewidth]{./results/CMP_new/synthesis_test/test_223_src.png}
\includegraphics[width=.19\linewidth]{./results/CMP_new/CMP_test/test/test_223_tgt.png}
\includegraphics[width=.19\linewidth]{./results/CMP_new/facades_pix2pix/images/224_fake_B.png}
\includegraphics[width=.19\linewidth]{./results/CMP_new/CMP_test/test/test_223_gen.png} \includegraphics[width=.19\linewidth]{./results/CMP_new/synthesis_test/test_223_des.png}\\ \vspace{1mm}

\includegraphics[width=.19\linewidth]{./results/CMP_new/synthesis_test/test_214_src.png}
\includegraphics[width=.19\linewidth]{./results/CMP_new/CMP_test/test/test_214_tgt.png}
\includegraphics[width=.19\linewidth]{./results/CMP_new/facades_pix2pix/images/215_fake_B.png}
\includegraphics[width=.19\linewidth]{./results/CMP_new/CMP_test/test/test_214_gen.png} \includegraphics[width=.19\linewidth]{./results/CMP_new/synthesis_test/test_214_des.png}\\ \vspace{1mm}

\includegraphics[width=.19\linewidth]{./results/CMP_new/synthesis_test/test_209_src.png}
\includegraphics[width=.19\linewidth]{./results/CMP_new/CMP_test/test/test_209_tgt.png}
\includegraphics[width=.19\linewidth]{./results/CMP_new/facades_pix2pix/images/210_fake_B.png}
\includegraphics[width=.19\linewidth]{./results/CMP_new/CMP_test/test/test_209_gen.png}
\includegraphics[width=.19\linewidth]{./results/CMP_new/synthesis_test/test_209_des.png} \\ \vspace{1mm}

\includegraphics[width=.19\linewidth]{./results/CMP_new/synthesis_test/test_202_src.png}
\includegraphics[width=.19\linewidth]{./results/CMP_new/CMP_test/test/test_202_tgt.png}
\includegraphics[width=.19\linewidth]{./results/CMP_new/facades_pix2pix/images/203_fake_B.png}
\includegraphics[width=.19\linewidth]{./results/CMP_new/CMP_test/test/test_202_gen.png}
\includegraphics[width=.19\linewidth]{./results/CMP_new/synthesis_test/test_202_des.png} \\ \vspace{1mm}
\caption{Generating images conditioned on architectural labels}	
\label{fig:supp_building4}
\end{figure*}

\begin{figure*}[h]
\centering
\includegraphics[width=.62\linewidth]{./results/CUHK/final_results.png}
\caption{Sketch interpolation}	
\label{fig:supp_face}
\end{figure*}

\begin{figure*}[h]
\centering	
\includegraphics[height=.6\linewidth]{./results/ZAP50k_test/UT_ZAP50K_Boots_larZAP50k_test/UT_ZAP50K_Boots_largege/test_000_src.png}\\
condition: edge images\\
\includegraphics[height=.6\linewidth]{./results/ZAP50k_test/UT_ZAP50K_Boots_large/test_000_des.png}\\
generated images by the policy-like and planner-like model\\
\caption{Generating shoes conditioned on edge images}	
\label{fig:supp_boot}
\end{figure*}

%\begin{table}[h]
%\centering
%\begin{small}
%\caption{Comparison with the baseline method for image inpainting.}%
%\label{tab:inpainting}
%\begin{tabular}{|l|c|c|} \hline 
%   & PSNR & SSIM \\ \hline \hline
%pixel2pixel \cite{isola2017image} & 19.3411 & 0.739 \\ 
%ours  & \textbf{20.4678} &  \textbf{0.767}\\ 
%\hline
%\end{tabular}
%\end{small}
%\end{table}

\begin{figure*}[h]
\centering	
\hspace{-4mm} images to be inpainted \hspace{14mm} GT \hspace{20mm} pixel2pixel \hspace{20mm} policy-like \hspace{14mm} planner-like \\
\includegraphics[width=.19\linewidth]{./results/CMP_recovery_test/test_094_src.png}
\includegraphics[width=.19\linewidth]{./results/CMP_recovery_test/test_094_tgt.png}
\includegraphics[width=.19\linewidth]{./results/CMP_recovery_pix2pix/095_fake_B.png}
\includegraphics[width=.19\linewidth]{./results/CMP_recovery_test/test_094_gen.png}
\includegraphics[width=.19\linewidth]{./results/CMP_recovery_test/test_094_des.png}\\
\includegraphics[width=.19\linewidth]{./results/CMP_recovery_test/test_007_src.png}
\includegraphics[width=.19\linewidth]{./results/CMP_recovery_test/test_007_tgt.png}
\includegraphics[width=.19\linewidth]{./results/CMP_recovery_pix2pix/008_fake_B.png}
\includegraphics[width=.19\linewidth]{./results/CMP_recovery_test/test_007_gen.png}
\includegraphics[width=.19\linewidth]{./results/CMP_recovery_test/test_007_des.png}\\
\includegraphics[width=.19\linewidth]{./results/CMP_recovery_test/test_017_src.png}
\includegraphics[width=.19\linewidth]{./results/CMP_recovery_test/test_017_tgt.png}
\includegraphics[width=.19\linewidth]{./results/CMP_recovery_pix2pix/018_fake_B.png}
\includegraphics[width=.19\linewidth]{./results/CMP_recovery_test/test_017_gen.png}
\includegraphics[width=.19\linewidth]{./results/CMP_recovery_test/test_017_des.png}\\
\includegraphics[width=.19\linewidth]{./results/CMP_recovery_test/test_021_src.png}
\includegraphics[width=.19\linewidth]{./results/CMP_recovery_test/test_021_tgt.png}
\includegraphics[width=.19\linewidth]{./results/CMP_recovery_pix2pix/022_fake_B.png}
\includegraphics[width=.19\linewidth]{./results/CMP_recovery_test/test_021_gen.png}
\includegraphics[width=.19\linewidth]{./results/CMP_recovery_test/test_021_des.png}\\

\includegraphics[width=.19\linewidth]{./results/CMP_recovery_test/test_082_src.png}
\includegraphics[width=.19\linewidth]{./results/CMP_recovery_test/test_082_tgt.png}
\includegraphics[width=.19\linewidth]{./results/CMP_recovery_pix2pix/083_fake_B.png}
\includegraphics[width=.19\linewidth]{./results/CMP_recovery_test/test_082_gen.png}
\includegraphics[width=.19\linewidth]{./results/CMP_recovery_test/test_082_des.png}\\

\includegraphics[width=.19\linewidth]{./results/CMP_recovery_test/test_020_src.png}
\includegraphics[width=.19\linewidth]{./results/CMP_recovery_test/test_020_tgt.png}
\includegraphics[width=.19\linewidth]{./results/CMP_recovery_pix2pix/021_fake_B.png}
\includegraphics[width=.19\linewidth]{./results/CMP_recovery_test/test_020_gen.png}
\includegraphics[width=.19\linewidth]{./results/CMP_recovery_test/test_020_des.png}
\caption{Example results of image inpainting}
\label{fig:supp_recovery}
\end{figure*}
